# Supplementary material for: Tunable mechanical coupling between driven microelectromechanical resonators
Source: arXiv:1607.04406 source file (2016-07-15)
Supplement: Supplementary file 1 [file Supplementary.pdf]

# Supplementary Materials for "Tunable mechanical coupling between driven microelectromechanical resonators"

G. J. Verbiest[1], D. Xu[1], M. Goldsche[1,2], T. Khodkov[1,2],
S. Barzanjeh[3,4], N. von den Driesch[2], D. Buca[2], and C. Stampfer[1,2]
[1]*JARA-FIT and 2nd Institute of Physics, RWTH Aachen University, 52074 Aachen, Germany*
[2]*Peter Grünberg Institute (PGI-8/9), Forschungszentrum Jülich, 52425 Jülich, Germany*
[3]*Institute for Quantum Information, RWTH Aachen University, 52056 Aachen, Germany and*
[4]*Institute of Science and Technology Austria, 3400 Klosterneuburg, Austria*

## CONTENTS

I. Theoretical model 2

II. Room temperature (RT) measurements 5

III. A device with fixed comb-drive 6

IV. Quality factors 7

References 8

# I. THEORETICAL MODEL

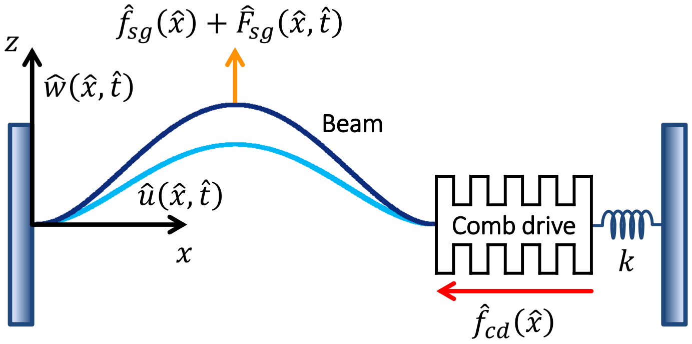


FIG. 1. The schematic of a silicon beam couples to comb-drive resonator. Here, $\hat{u}(\hat{x})$ and $\hat{w}(\hat{x})$ are the displacement components along the $x$ (in-plane) and $z$ (out of-plane) directions.

In this section, we derive the equations of motion and the dynamic response governing finite-amplitude transverse vibrations of a homogeneous, isotropic, geometrically imperfect silicon beam with length $l$ and mass per unit length $m$ which in one site is axially coupled to a movable comb-drive with total mass $M$. We let $\hat{u}(\hat{x})$ and $\hat{w}(\hat{x})$ be the displacement components, at position $\hat{x}$, along the $x$ (in-plane) and $z$ (out of-plane) directions, respectively (see Fig. 1), where the hat designates dimensional variables. The total potential energy describing an Euler-Bernoulli beam undergoing transverse displacements is given by,

$$V = \frac{1}{2}EA\int_0^\ell \epsilon_s^2 \mathrm{d}\hat{x} + \frac{1}{2}EI\int_0^\ell (\hat{w}'')^2\,\mathrm{d}\hat{x} - \int_0^\ell \hat{f}_{sg}\,\hat{w}\,\mathrm{d}\hat{x} + \hat{f}_{cd}\,\hat{u}(\ell,\hat{t}) + \frac{1}{2}k\,\hat{u}^2(l,\hat{t}), \tag{1}$$

where $\ell$ is the span of the beam, $A$ is the cross section area, and $I$ is the area moment of inertia. For a rectangular area with width $b$ and height $h$, the area moment of inertia is $I = bh^3/12$. Furthermore, $E$ is the Young's modulus, $\hat{f}_{sg}$ is a static transverse side-gate load, $\hat{f}_{cd}$ is a static comb-drive end load applied at $\hat{x} = l$, and the prime denotes differentiation with respect to $\hat{x}$. We consider the comb-drive as a mass-spring configuration (with mechanical stiffness $k$) that is attached to the beam at $\hat{x} = l$, see Fig 1. The first term of Eq. (1) describes the stretching energy of the beam, the second term accounts for bending energy, the third and forth terms stand for the external transverse and axial driven forces, respectively, and the last term describes the potential energy of the comb-drive (spring) coupled to the beam. Here, $\epsilon_s = \frac{\mathrm{d}\hat{s}}{\mathrm{d}\hat{x}} - 1$ is the strain accounting for stretching of the midplane surface of the beam with,

$$\mathrm{d}\hat{s} = \sqrt{(1+\hat{u}')^2 + \hat{w}'^2}\,\mathrm{d}\hat{x}, \tag{2}$$

represents the length of a line element of the centerline of the imperfect beam in the deformed configurations. By expanding Eq. (2) to second order and considering $\hat{u}'^2 \ll \hat{w}'^2$, the strain of the beam reduces to,

$$\epsilon_s \simeq \hat{u}' + \frac{1}{2}\hat{w}'^2. \tag{3}$$

Finally, the total kinetic energy of the silicon beam coupled to the comb-drive is,

$$T = \frac{1}{2}\int_0^\ell m\left(\dot{\hat{u}}^2 + \dot{\hat{w}}^2\right)\mathrm{d}\hat{x} + \frac{1}{2}M\dot{\hat{u}}^2(l,\hat{t}). \tag{4}$$

By using Hamilton's extended principle we can find the equations of motion,

$$\delta\int_{\hat{t}_1}^{\hat{t}_2}(T-V)\mathrm{d}\hat{t} + \int_{\hat{t}_1}^{\hat{t}_2}\int_0^l \hat{F}_{sg}\left(\hat{x},\hat{t}\right)\delta\hat{w}\mathrm{d}\hat{t} = 0, \tag{5}$$

where $\hat{F}_{sg}\left(\hat{x},\hat{t}\right)$ is a nonconservative transverse distributed load. Substituting Eqs. (1)-(4) into Eq. (5) and performing the pertinent variations and integrations yields the following three nonlinear coupled equations,

$$m\ddot{\hat{u}} - EA\epsilon_s' = 0, \tag{6a}$$

$$m\ddot{\hat{w}} + EI\hat{w}'''' - EA(\epsilon_s\hat{w}')' = \hat{f}_{sg} + \hat{F}_{sg}(\hat{x},\hat{t}), \tag{6b}$$

$$M\ddot{\hat{u}}_l + k\hat{u}_l + EA\epsilon_s = \hat{f}_{cd}, \tag{6c}$$

where $\hat{u}_l \equiv \hat{u}(l,\hat{t})$ represents the horizontal (in-plane) displacement at $\hat{x} = l$. Here, we consider an Euler-Bernoulli beam in which the shear deformation, longitudinal inertia, and rotary inertia of the beam are negligible. The second assumption allows the elimination of the beam longitudinal degree of freedom, $\ddot{u} = 0$ in Eq. (6a) which results in $\epsilon_s' \sim 0$. This approximation implies that the total stretching strain field along the centerline of the beam is constant. Making use of this approximation along with assuming $\hat{u}(0) = 0$ and integrating Eq. (3) from $\hat{x} = 0$ to $\hat{x} = l$, yields,

$$\epsilon_s = \frac{\hat{u}_l}{l} + \frac{1}{2l}\int_0^l \hat{w}'^2 \mathrm{d}\hat{x}. \tag{7}$$

Therefore, the Eqs. (6) can be simplified to,

$$m\ddot{\hat{w}} + EI\hat{w}'''' - \frac{EA}{l}\Big(\hat{u}_l + \frac{1}{2}\int_0^l \hat{w}'^2 \mathrm{d}\hat{x}\Big)\hat{w}'' = \hat{f}_{sg}(\hat{x}) + \hat{F}_{sg}(\hat{x},\hat{t}), \tag{8a}$$

$$M\ddot{\hat{u}}_l + \Big(k + \frac{EA}{l}\Big)\hat{u}_l + \frac{EA}{2l}\int_0^l \hat{w}'^2 \mathrm{d}\hat{x} = \hat{f}_{cd}(\hat{x}). \tag{8b}$$

Note, however that, the total side-gate force $\hat{F}_T(\hat{x},\hat{t}) = \hat{f}_{sg}(\hat{x}) + \hat{F}_{sg}(\hat{x},\hat{t})$, can be expressed in term of the capacitance between the beam and side-gate $C_{sg}$, i.e., $\hat{F}_T(\hat{x},\hat{t}) = -\frac{1}{2}\frac{\partial C_{sg}}{\partial \hat{w}}V_{sg}^2$ where $V_{sg} = V_{sg}^{DC} + V_{sg}^{AC}\cos(\omega\hat{t})$ is the applied voltage on the side-gate. The similar expression relates the comb-drive force to the effective capacitance between the fingers of the comb-drive $\hat{f}_{cd}(\hat{x}) = -\frac{1}{2}\frac{\partial C_{cd}}{\partial \hat{w}}V_{cd}^2$ where $V_{cd}$ is the voltage applied on the comb-drive.

To obtain the equations governing vibrations around the nonlinear equilibrium $w_{DC}(\hat{x})$ and $\hat{y}_0$, we let,

$$\hat{w}(\hat{x},\hat{t}) = \hat{w}_{DC}(\hat{x}) + \hat{v}(\hat{x},\hat{t}), \tag{9a}$$

$$\hat{u}_l(\hat{t}) = \hat{y}_0 + \hat{z}(\hat{t}). \tag{9b}$$

where $\hat{v}(\hat{x},\hat{t})$ represents the dynamic deflection of the beam and $\hat{z}(\hat{t})$ demonstrates the dynamical vibration of the comb-drive. It is, however, convenient to rescale the relevant quantities into dimensionless parameters,

$$u = \frac{\hat{u}}{r},\quad w = \frac{\hat{w}}{r},\quad x = \frac{\hat{x}}{l},\quad t = \hat{t}\Omega,\quad \begin{pmatrix} f_{sg}(\hat{x}) \\ F_{sg}(x,t) \end{pmatrix} = \frac{l^4}{rEI}\begin{pmatrix} \hat{f}_{sg}(x) \\ \hat{F}_{sg}(\hat{x},\hat{t}) \end{pmatrix},\quad f_{cd}(x) = \frac{\hat{f}_{cd}(\hat{x})l^2}{EI}, \tag{10}$$

where $r = \sqrt{I/A}$ denotes the radius of gyration of the cross section that is a measure of the slenderness of the beam and $\Omega = \sqrt{\frac{EI}{ml^4}}$ is the resonance frequency of the first vibrational mode of a beam's free oscillation according to the Euler-Bernoulli beam theory.

By substituting Eqs. (9) into Eqs. (8) and dropping the time-dependent terms, one can find the equation of motion describing the static response of the beam,

$$w_{DC}''''(x) - T_{\text{eff}}\, w_{DC}''(x) = f_{sg}, \tag{11}$$

where,

$$T_{\text{eff}} = f_{cd} + \frac{k_r l}{2}\int_0^1 w_0'^2 \mathrm{d}x, \tag{12}$$

demonstrates the total tensile force acting on the beam in which $k_r = \frac{klr^2}{EI}$ denotes the rescaled spring constant.

The solution of Eq. (11) is given by,

$$w_0(x) = a_0\psi(x), \tag{13}$$

where $\psi(x) = \sqrt{\frac{2}{3}}(1 - \cos 2\pi x)$, with $\int_0^1 \psi^2(x)\, dx = 1$, evaluates the static shape of the beam and,

$$a_0 = \sqrt{\frac{3}{2}}\frac{f_{sg}}{16\xi T_{\text{eff}}}\left(\xi - 4\tanh\frac{\xi}{4}\right). \tag{14}$$

gives the maximum displacement of the beam's center in which $\xi^2 = T_{\text{eff}}$.

The dynamics of the system is fully described by the solutions of time-dependent equations (8). These equations are nonlinear and in general we cannot solve them analytically. Therefore, we limit our analysis to the case where the amplitude of dynamical deflection is much smaller than the static deflection of the beam i.e., $v(x,t) \ll w_{DC}(x)$. However, without

lose of generality we expand the dynamical deflection of the beam in terms of basis function $\psi(x)$, i.e $v(x,t) = v(t)\psi(x)$ where $v(t)$ describes the time-dependent amplitude of the beam's vibration. As a result Eqs. (9), after rescalling, reduce to,

$$\begin{aligned} w(x,t) &= [a_0 + v(t)]\psi(x), \\ u_l(t) &= y_0 + z(t). \end{aligned} \tag{15}$$

By substituting Eqs. (15) into the nonlinear equations (8) and dropping the nonlinear terms proportional to $O(v^2)$, we obtain the following nonhomogeneous differential equation governing linear vibrations around the nonlinear equilibrium configuration $\psi(x)$,

$$\ddot{v} + \lambda_1 v + \Gamma u_l = \sqrt{\frac{2}{3}} F(t) \sim 0, \tag{16a}$$

$$\mu \ddot{u}_l + \lambda_2 u_l + \Gamma v = 0, \tag{16b}$$

in which the time dependent part of the transverse load $F(t)$ is regarded as a very small fluctuation on the static transverse load as there can be orders of magnitudes difference between them. Thus, $F(t)$ is neglected for simplifying the calculation below. The coefficients in these equations are defined as,

$$\lambda_1 = \frac{16\pi^4}{3} + \frac{4\pi^2}{3}\left[f_{cd} + \frac{4\pi^2}{3} a_0^2 \left(1 + \frac{k_r}{2}\right)\right] - \frac{f_{sg}}{2}, \tag{17a}$$

$$\lambda_2 = \frac{l^2}{r^2}\left(k_r + 1\right), \tag{17b}$$

$$\Gamma = \frac{4\pi^2}{3} \frac{l}{r} a_0, \tag{17c}$$

$$\mu = \frac{M}{mAl}, \tag{17d}$$

among which $\Gamma$ denotes the coupling rate between the transversal mode of the beam and the axial mode of the comb-drive.

By solving the Eqs. (17) we can find the response frequencies of the system. To do this we apply the Fourier transform on Eqs. (17), which gives,

$$-\omega^2 v + \lambda_1 v + \Gamma u_l = 0, \tag{18a}$$

$$-\mu\omega^2 u_l + \lambda_2 u_l + \Gamma v = 0. \tag{18b}$$

The eigenvalues of the above equations gives two effective frequencies describing the response frequencies of the coupled system,

$$\omega_1 = \sqrt{\frac{\mu\lambda_1 + \lambda_2 - \sqrt{4\Gamma^2\mu + (-\mu\lambda_1 + \lambda_2)^2}}{2\mu}}, \tag{19a}$$

$$\omega_2 = \sqrt{\frac{\mu\lambda_1 + \lambda_2 + \sqrt{4\Gamma^2\mu + (-\mu\lambda_1 + \lambda_2)^2}}{2\mu}}. \tag{19b}$$

## II. ROOM TEMPERATURE (RT) MEASUREMENTS

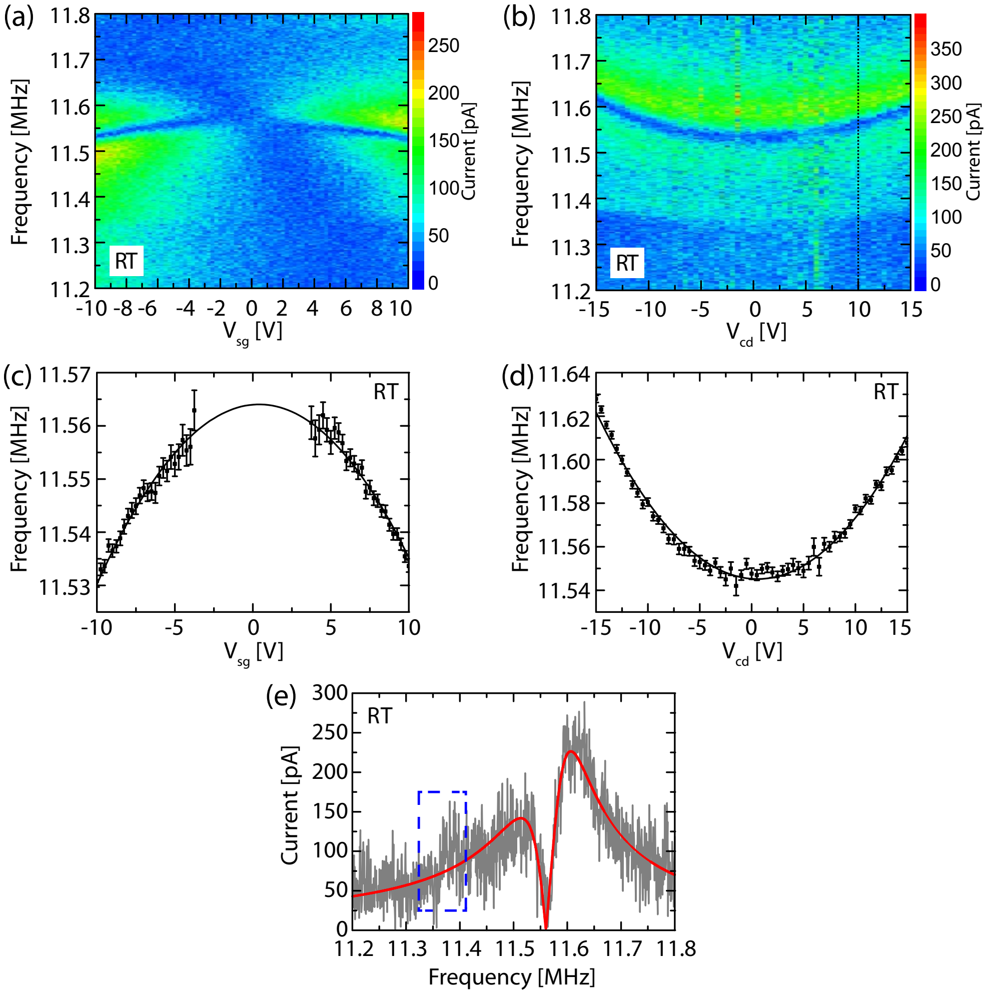


FIG. 2. A measured down-mixed current as functions of (a) the applied $V_{sg}^{DC}$ at $V_{cd} = 10$ V and (b) $V_{cd}$ at $V_{sg}^{DC} = 10$ V at RT. The extracted resonance frequencies of (a) and (b) are shown in (c) and (d) with quadratic fits, respectively. The vertically dashed black line in (b) indicates the curve shown in (e). The red line is the fit. The region in the RT spectra indicated with the blue box in (e) does show a reproducible step in current hinting towards the existence of a second resonance at RT as well. This step is clearly visible in the RT map (b) as a function of applied $V_{cd}$.

## III. A DEVICE WITH FIXED COMB-DRIVE

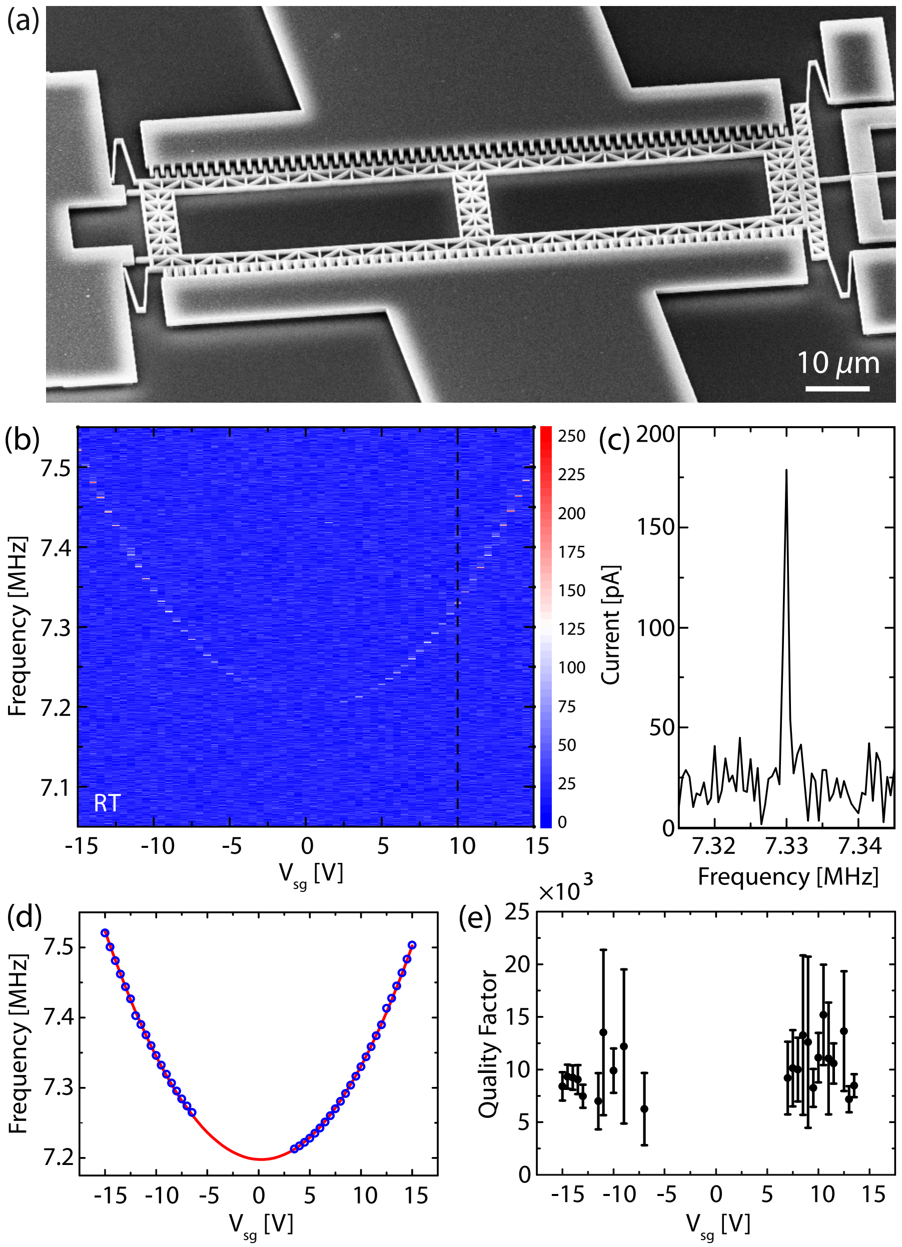


FIG. 3. To prove the strongly coupled oscillations in our device, we measure another device of which the comb-drive actuator is fixed. (a) the SEM image shows that the comb-drive touches the underlying silicon layer and thus can not move. (b) the down mixed current as a function of side-gate voltage $V_{sg}$ and frequency of a fabricated device with a fixed comb-drive. The vertically dashed black line indicates the applied $V_{sg}$ of the raw data curve in (c). We observed only a single resonance for this device. The tunability of the resonance frequencies shows clear quadratic behavior in (d). The red line shows the quadratic fit. (e) the quality factors ($Q \sim 10\ 000$) is approximately 10 to 100 times higher than that for the device represented on Fig. 4 (see Suppl. Mat. IV). This suggests that a significant amount of energy is transferred from the silicon beam into the comb-drive actuator and vice versa.

## IV. QUALITY FACTORS

The quality factors corresponding to the strongly coupled oscillators at ∼ 300 K (RT) and 2.3 K are summarized in Fig. 4. For the given device geometry, we estimate the quality factor due to clamping losses [1] to be ∼ 360 and to thermal dissipation [2] to be $10^9$ and thus negligible. Apart from these two mechanisms, it is expected that surface dissipation [3] also plays a role. At RT, the extracted quality factor is far below the one estimated from clamping losses. Therefore, we conclude that the quality factor at RT is limited by surface dissipation. Additional evidence for this is found from the quality factor dependence on the applied (surface) stress via $V_{sg}$ and $V_{cd}$. The quality factor for surface dissipation should range from ∼ 150 to ∼ 250 to let the total quality factor approach the experimental data. By cooling down the device to 2.3 K, the quality factor increases to ∼ 400 for the HSM and ∼ 1200 for the LSM. Surprisingly, the quality factor does not depend on the applied (surface) stress anymore, which suggest that the quality factor is completely determined by clamping losses. As the quality factor for the device with the fixed comb-drive actuator was ∼ 10 000, a significant part of the vibrational energy of the silicon beam is, hence, transferred into the comb-drive actuator, which is an independent (energy) argument for a system of two strongly coupled resonators.

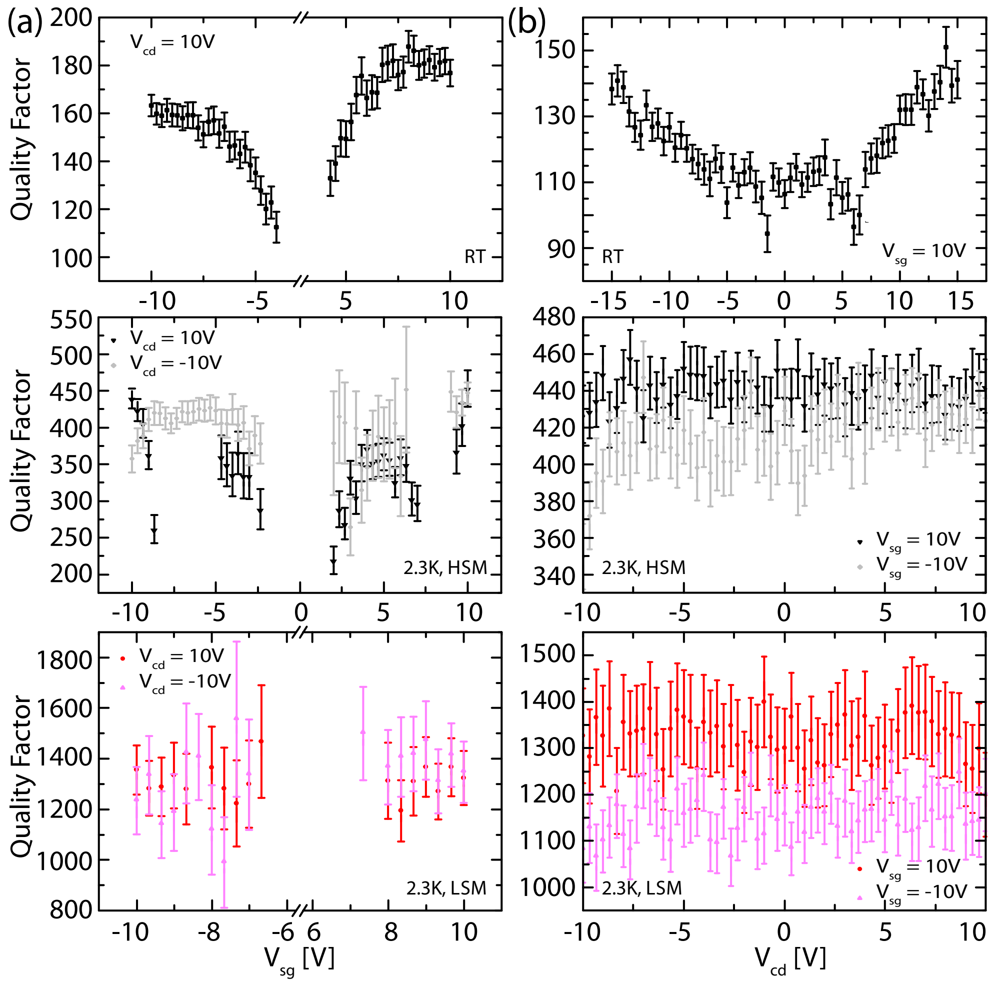


FIG. 4. The extracted quality factor of the resonance frequencies as a function of (a) $V_{sg}$ and (b) $V_{cd}$. From top to bottom, the panels show the quality factor at RT and at 2.3 K for the HSM, and only at 2.3 K for the LSM. At RT, the quality factor increases with $V_{sg}$ until $|V_{sg}| = 8$ V after which it saturates, whereas the quality factor appears to increase linearly with $V_{cd}$ when $|V_{cd}|$ is larger than 5 V.

[1] Z. Hao, A. Erbil, and F. Ayazi, Sensor. Actuat. A-Phys. **109**, 156 (2003).
[2] R. Lifshitz and M. Roukes, Phys. Rev. B **61**, 5600 (2000).
[3] J. Yang, T. Ono, and M. Esashi, Sensor. Actuat. A-Phys. **82**, 102 (2000).
